# Supplementary material for: Semi-Supervised Training to Improve Player and Ball Detection in Soccer
Source: arXiv:2204.06859 source file (2022-04-14)
Supplement: Supplementary file 1 [file 6_supplementary.tex]

\section{Supplementary Material}
